# Supplementary material for: How do Mixture Density RNNs Predict the Future?
Source: arXiv:1901.07859 ancillary file (2019-01-23)
Supplement: Supplementary file 1 [file supplementary_info.pdf]

# How do Mixture Density RNNs Predict the Future? - Supplementary Material

Kai Olav Ellefsen [1] Charles Patrick Martin [1 2] Jim Torresen [1 2]

## 1. World Model Details

### 1.1. Overall Structure

Our World Model setup closely follows that employed by (Ha and Schmidhuber, 2018) for modeling the VizDoom TakeCover scenario. The main difference is that we train only the visual (V) and memory (M) component of our World Model. A controller (C) is not necessary, since our focus is on analyzing predictions, and not on using them to guide control. The overall setup of the World Model is given in the main paper - we here present the details of each component and their parameters.

### 1.2. Data collection

Data to train the World Model is collected by an agent carrying out random actions in the VizDoom TakeCover scenario. In each timestep, the agent takes a random action (move left, move right or stand still), and we store the resulting image of the environment, down-sampled to 64x64, together with the action – which will later be used to train the vision and memory modules. In order to get a relatively stable motion, we repeat the random action a number of times, sampled uniformly between 1 and 10. We collect 2000 of these episodes for training, each episode lasting until the agent is killed (due to being hit by fireballs), or until it has reached 2100 timesteps (1 minute of real-time play).

### 1.3. Visual Module: VAE

Our variational autoencoder follows the layout from (Ha and Schmidhuber, 2018). It takes single images from the VizDoom scenario as training data and learns a compressed representation of these. Images from the game are down-sampled to 64x64x3 (the latter representing color components) before training.

The VAE consists of 4 convolutional layers, encoding the input to lower-dimensional vectors $\mu_{vae}$ and $\sigma_{vae}$, both real-valued of length 64. A length 64 latent vector $z$ is sampled from a normal distribution parameterized $\mu_{vae}$ and $\sigma_{vae}$. $z$ is finally sent through 4 deconvolution layers to reconstruct the image.

Training the VAE consists in presenting the same images as inputs and target outputs, and minimizing two loss components: 1) The reconstruction loss, measured as the binary cross-entropy between the input and output, and 2) a regularization loss, measured via the KullbackLeibler divergence. Together, the two tend to result in models that can both compress and reconstruct inputs, and that also have a structured latent space. Ha and Schmidhuber demonstrated that this VAE, trained on images from games, learned to form a latent space where certain variables correspond to meaningful dimensions of variation in the input images, such as the curvature of the road in a car-racing game. For further details, we refer the reader to (Ha and Schmidhuber, 2018) and our online implementation [1].

### 1.4. Memory Module: MD-RNN

After training the VAE, we can generate latent vectors $z$ for all collected frames, allowing us to train the RNN on sequences of vectors of length 64 rather than 64x64x3 images. The memory module consists of a single layer of 256 LSTM (Hochreiter and Schmidhuber, 1997) units, which learn to model the probability distribution over the next $z$-vector given the current history of latent vectors and the current action. This probability is modeled by a mixture of multivariate Gaussian distributions, that is, a probability distribution composed of several (5 in our case) weighted multivariate Gaussian distributions. Transformation of the RNN output to the mixture distribution parameters is handled by a mixture density network (Bishop, 1994) (MDN). The combined MD-RNN network transforms latent vectors $z$, into the parameters $\boldsymbol{\theta}$, of this distribution, consisting of weights ($\boldsymbol{\pi}(z)$), means ($\boldsymbol{\mu}_k(z), k = 1, \ldots, 5$), and covariance matrices ($\boldsymbol{\Sigma}_k(z), k = 1, \ldots, 5$) of output mixture distribution. To make the loss function on this MD-RNN tractable, the covariance matrices are limited to be diagonal.

During training, the RNN takes as input 60 z-vectors ($\boldsymbol{z}$) and associated actions in a sequence and produces as outputs the parameters of the mixture distribution that could predict the next z-vector for each of them. That is, given $\boldsymbol{z}$ for timestep 1-60, probability distribution predictions are generated for

[1]Department of Informatics, University of Oslo, Norway [2]RITMO, University of Oslo, Norway. Correspondence to: Kai Olav Ellefsen <uio>.

[1]http://doi.org/10.5281/zenodo.2539145

timestep 2-61. The actual observed z-vectors for those timesteps are used as targets ($\boldsymbol{t}$), and the loss is calculated from the likelihood of observing these targets in the mixture distributions calculated from $\boldsymbol{z}$. The probability density function (PDF) of the mixture distribution is applied to calculate the loss:

$$p(\boldsymbol{t}|\boldsymbol{z}) = \sum_{k=1}^{5} \pi_k(\boldsymbol{z})\mathcal{N}(\boldsymbol{\mu}_k(\boldsymbol{z}), \boldsymbol{\Sigma}_k(\boldsymbol{z}); \boldsymbol{t}) \qquad (1)$$

Our code applies the TensorFlow Probability library (Dillon et al., 2017) to calculate the loss function of the MD-RNN. When training our system, examples are extracted with a window of 60 frames as explained above and a hop size of 5 frames.

After training and during inference, the RNN takes a single z-vector as input and produces the mixture distribution parameters $\boldsymbol{\theta}$ as output. From this distribution, one or more $z$-vectors can be sampled. To predict further into the future, samples from this distribution are fed back into the RNN as input, allowing the RNN to "dream" long sequences of z-vectors.

Our formulation differs from Ha and Schmidthuber's (2018), in that whereas those authors used 60 mixture distributions of 1D Gaussians to model the VAE's latent space, we use a single mixture of 60-dimensional Gaussian distributions. While their approach worked for playing games, it does not allow the analysis of the latent-space predictions that we have engaged with in this research since each dimension of the latent space is governed by a separate mixture distribution. Our formulation also generates coherent dreams, and has the advantage that the mixing parameters, $\boldsymbol{\pi}$, govern which multivariate Gaussian is used to sample future $z$-vectors, allowing us to investigate how aspects of the world are predicted by the MD-RNN. Note that the number of mean ($\mu$) and scale ($\sigma$) parameters we generate are the same as Ha and Schmidhuber, however we generate only 5 weights ($\pi$) while they generate $5 \times 60$.

### 1.5. Parameters

Parameters of the World Models we trained are found in Table 1. Particular to the MDN are the $\pi$ and $\sigma$ temperatures which govern how much randomness there is in sampling between and within the Gaussian components, respectively. We define $\pi$-temperature to be the standard adjustment to the softmax distribution defined by the $\boldsymbol{\pi}$s, and $\sigma$-temperature to be a linear scaling of the scales $\boldsymbol{\sigma}$ that define the diagonal covariance matrices $\boldsymbol{\Sigma}$.

The $\pi$ temperature we have chosen gives some freedom to explore different mixtures when they are weighted evenly, and the low $\sigma$ temperature reduces the randomness when sampling from a specific mixture. In practice, we found a low $\sigma$ temperature to be necessary to produce coherent predictions similar to the training data. Note that these sampling temperatures only affect the generation of new predictions, and are not used during training.

| **Parameter** | Value |
|---|---|
| Training data size | 2000 episodes |
| Max. episode length | 2100 timesteps |
| VAE training epochs | 10 |
| VAE batch size | 100 |
| Number of MDN-mixtures | 5 |
| RNN training epochs | 1000 |
| RNN batch size | 256 |
| MDN $\pi$ temperature | 1.0 |
| MDN $\sigma$ temperature | 0.01 |

*Table 1.* Parameters of the World Model.

## 2. Automatically Identifying Events in Predictions

When measuring the relationship between MDN-components and predicted events, we need to identify events in predicted frames. Ideally, this could be done manually for the highest-quality measurements, but this is infeasible due to the large amount of frames that needed to be analyzed in our experiments (thousands for the results presented herein). We therefore developed some simple image analysis methods to automate the identification of events. Since the world we are modeling is quite simple, we can rely on some relatively straightforward analyses of images to identify fireballs, explosions, monsters and walls.[2]

| **Parameter** | Value |
|---|---|
| Fireball Threshold | 0.65 |
| Monster Threshold | 0.2 |
| Wall Threshold | 0.39 |

*Table 2.* Parameters of the methods for automatically identifying events. See how they are used below.

### 2.1. Identifying explosions

Explosions are large, bright spots that fill up a significant portion of the image. A challenge in classifying these is that fireballs near the agent are also large and bright. However, an observation that made the classification of explosions

[2]A Jupyter notebook demonstrating the methods is available at https://github.com/kaiolae/WorldModels/blob/master/notebooks/AutomaticallyCountingMonstersAndFireballs-Permalink.ipynb

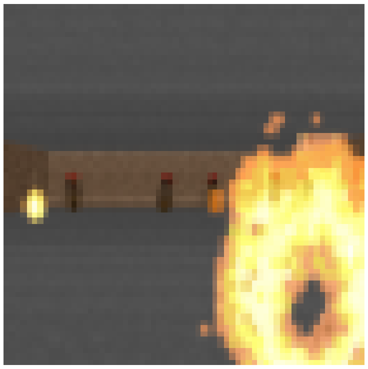

(a) A frame with an explosion

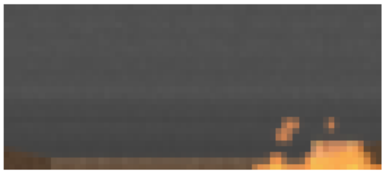

(b) The top part of the explosion frame

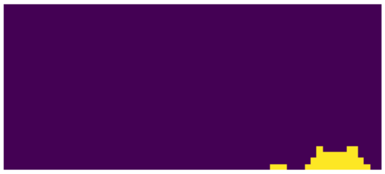

(c) Thresholded version of image in b.

*Figure 1.* Detecting an explosion in a dream uses only the top part of the image, since fireballs never extend to this part.

easier is that explosions in the training data always extend to the top half of the screen. Fireballs on the other hand, always stay in the lower half of the screen. To check if an explosion is present, we therefore 1) cut out the top part of the image (pixel rows 0 to 28), and then 2) check if there are any objects with a brightness above the Fireball Threshold (Table 2) value in this part.

If an explosion is present, we do not try to identify other elements in the scene, since explosions are large and tend to occlude important elements (e.g. fireballs and monsters). Counting fireballs and monsters would therefore likely miss some elements.

### 2.2. Counting fireballs

Counting fireballs is relatively straightforward, since their intensity is higher than all other elements in the scene. The only other object they could be confused with are explosions, but, as explained above, when explosions are detected, we do not count other elements in the scene.

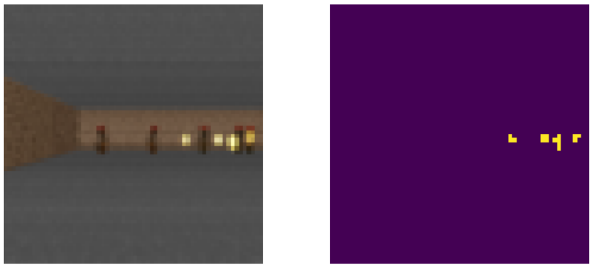

(a) A frame with 4 fireballs (b) Thresholded frame

*Figure 2.* Counting fireballs consists of thresholding the image, before counting connected components.

Counting fireballs is done by 1) thresholding the scene according to the Fireball Threshold (Table 2), before 2) counting the number of connected components. An example is shown in Figure 2.

### 2.3. Counting monsters

Counting monsters is difficult, since monsters are frequently occluded entirely or partially by fireballs. To minimize this problem, we count monsters by focusing only on the slice of the image that contains monsters' heads. Since monsters only move side-to-side, this is always a fixed part of the image. This helps avoid counting one monster as two, in cases where their heads and feet are separated by a fireball.

After separating out this slice of the image, counting monsters is done by 1) extracting only the green-component of the image (which is the best one for separating monsters from other dark items), 2) thresholding the green-only image according to the Monster Threshold (Table 2), keeping only the darkest components, and 3) counting connected components. See Figure 3 for an example.

### 2.4. Checking if we are near a wall

Checking if we are near a wall is straightforward, since walls have very different colors than the ceiling and floor. To check if we are near a wall on the right-hand side, we simply measure the average value of the red-component of the 10 top pixels on the rightmost column of the image. If they are above a threshold (Wall Threshold in Table 2), we are near a wall. The red-component of the gray ceiling and the brown walls is so different, that this was found to be a very robust check.

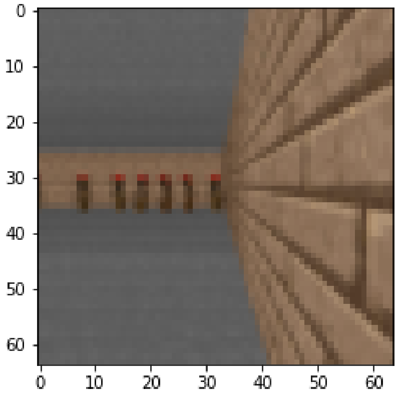

(a) A frame with 6 monsters

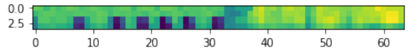

(b) The slice containing monsters' heads

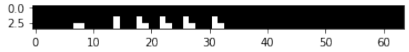

(c) Thresholded version of image in b.

*Figure 3.* Counting monsters is facilitated by focusing only on the slice of the image where monsters' heads are. Since monsters are darker than other components, thresholding by image intensity helps counting them.

## References

D. Ha, J. Schmidhuber, Recurrent World Models Facilitate Policy Evolution, in: S. Bengio, H. Wallach, H. Larochelle, K. Grauman, N. Cesa-Bianchi, R. Garnett (Eds.), Advances in Neural Information Processing Systems 31, Curran Associates, Inc., 2018, pp. 2451–2463.

S. Hochreiter, J. Schmidhuber, Long Short-Term Memory, Neural Computation (1997).

C. M. Bishop, Mixture Density Networks, Technical Report NCRG/97/004, Neural Computing Research Group, Aston University, 1994.

J. V. Dillon, I. Langmore, D. Tran, E. Brevdo, S. Vasudevan, D. Moore, B. Patton, A. Alemi, M. D. Hoffman, R. A. Saurous, Tensorflow distributions, CoRR abs/1711.10604 (2017).
